# Supplementary material for: Imaging Oxygen Defects and their Motion at a Manganite Surface
Source: arXiv:1110.0636 ancillary file (2011-10-04)
Supplement: Supplementary file 1 [file Supplementary_Material.pdf]

# Imaging Oxygen Defects and their Motion at a Manganite Surface: Supplementary Material

B. Bryant[1], Ch. Renner[2], Y. Tokunaga[3], Y. Tokura[3,4,5], G. Aeppli[1]

[1]*London Centre for Nanotechnology and Department of Physics and Astronomy, University College London, London WC1E 6BT, UK*
[2]*Department of Condensed Matter Physics, University of Geneva, 24 Quai Ernest-Ansermet, CH-1211 Geneva 4, Switzerland*
[3]*Multiferroic Project, ERATO, Japan Science and Technology Agency (JST), Wako, 351-0198, Japan*
[4]*Cross-Correlated Materials Research Group (CMRG), RIKEN, Advanced Science Institute, Wako, 351-0198, Japan*
[5]*Department of Applied Physics, University of Tokyo, Bunkyo-ku, Tokyo 113-8656, Japan*

## Supplementary Figures

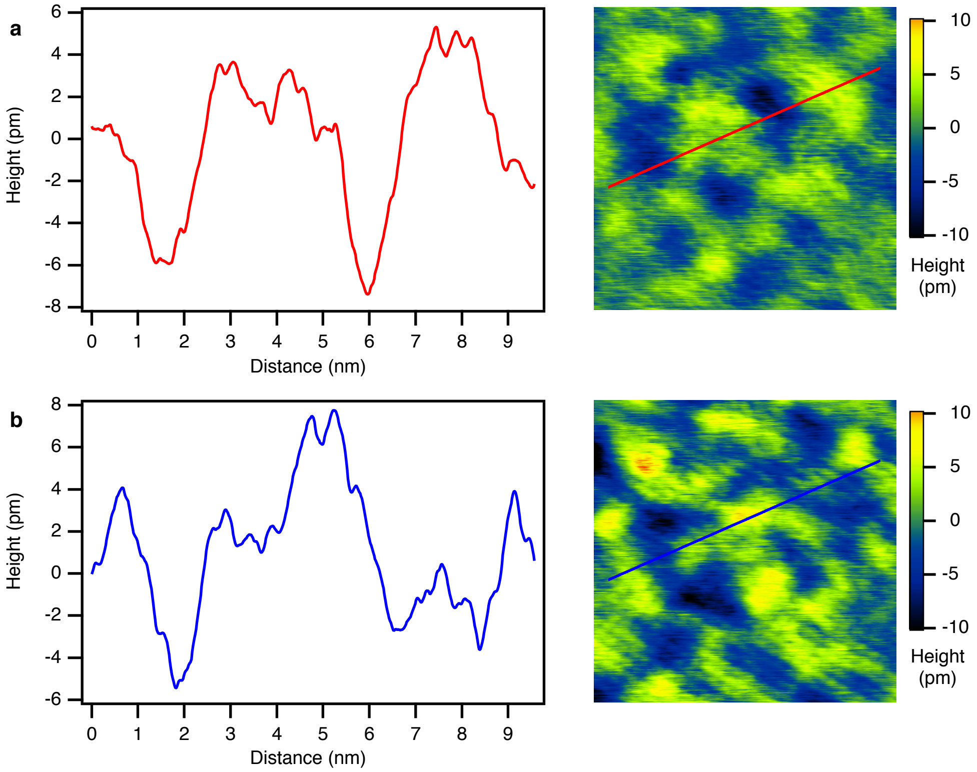


Supplementary Figure S1: **Bias dependence of $PrSr_2Mn_2O_7$ surface inhomogeneities.** (a) 10 x 10 $nm^2$ empty state (+0.8 V, 100 pA) topographic image of $PrSr_2Mn_2O_7$ collected at 78 K. Surface inhomogeneities are visible: the structure is irregular but has an in-plane length scale of 3-4 nm and an amplitude of $\approx$ 20 pm peak-peak. (b) Image collected simultaneously on the same area in filled states (-0.8 V, 100 pA). Sections are shown for both images: some inhomogeneous features remain the same between filled and empty states, whilst others change. This implies that both topographic and electronic components contribute to the imaging contrast. The electronic component is most likely related to the inhomogeneous distribution of $Mn^{3+}$ and $Mn^{4+}$ ions in the surface layers, or to the distribution of $Pr^{3+}$ and $Sr^{2+}$ ions, or a combination of these factors. Positive and negative bias STM images have been collected simultaneously, by using dual bias mode to interlace images taken at two different biases. Images have been aligned by cross-correlation to correct for the effect of piezo hysteresis.

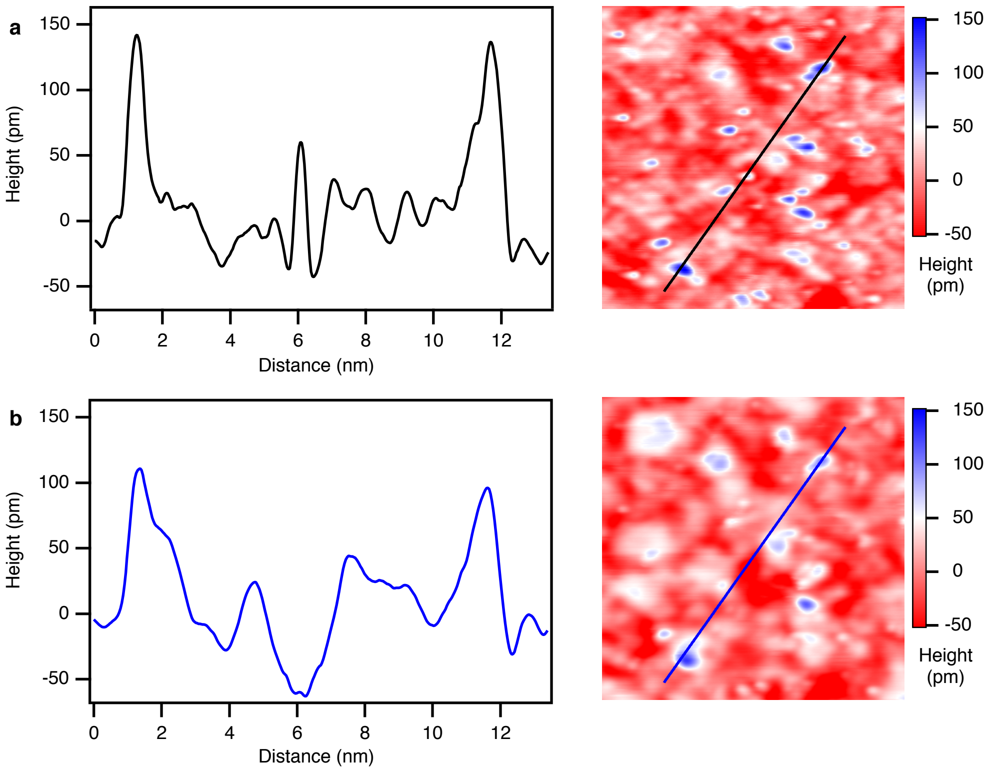


Supplementary Figure S2: **Bias dependence of adatom imaging.** (a) 12 x 12 nm$^2$ filled state (-0.8 V, 100 pA) topographic image of $PrSr_2Mn_2O_7$ collected at 78 K, showing adatoms and vacancies. (b) Simultaneously acquired empty state image (+0.8 V, 100 pA). Sections are shown for both images: The same adatoms are visible in both filled and empty states. This indicates that the adatoms are physical entities rather than purely electronic contrast features. Adatoms are more clearly resolved in filled states than in empty states: in filled states the adatoms have a height of around 0.14 nm, whilst in empty states the height is around 0.11 nm. The increased contrast in filled states can be explained if the adatoms are negatively charged oxygen, since this will enhance the filled state tunnel current. Positive and negative bias STM images have been collected simultaneously, by using dual bias mode to interlace images taken at two different biases. Images have been aligned by cross-correlation to correct for the effect of piezo hysteresis.

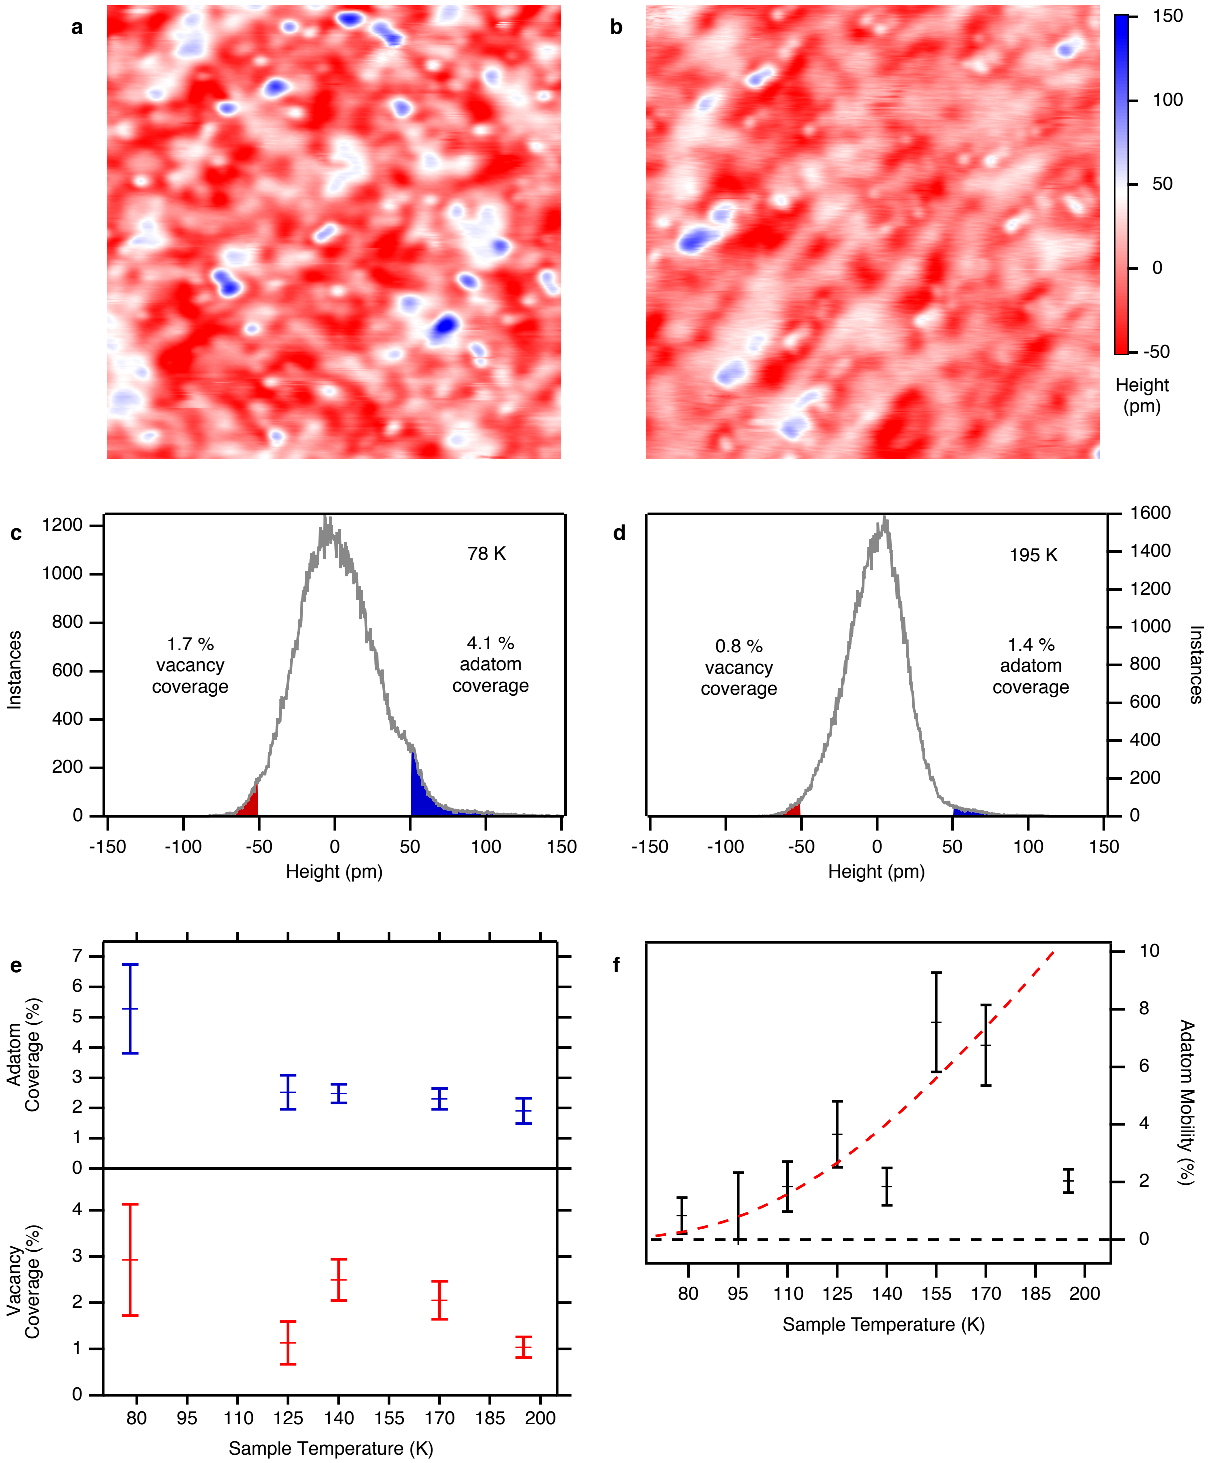


Supplementary Figure S3: **Temperature dependence of adatom and vacancy coverage, and adatom mobility.** (a) 20 x 20 $nm^2$ STM micrograph collected at 78 K (b) 20 x 20 $nm^2$ STM micrograph at 195 K. Both +0.8 V, 100 pA. (c) and (d) histograms of (a) and (b) respectively. Areas below -50 pm represent vacancies (shaded red): areas above +50 pm represent adatoms (shaded blue). (e) Adatom and vacancy image coverage, as a function of sample temperature. Error bars represent one standard deviation. (f) Mean fraction of mobile adatoms, per frame, as extracted from time series of images, as a function of sample temperature. Error bars represent one standard error. The dashed line is a fit of the form $exp(-E_A/k_bT)$. $E_A$ = 480 ± 170 K. See Supplementary Discussion for full details.

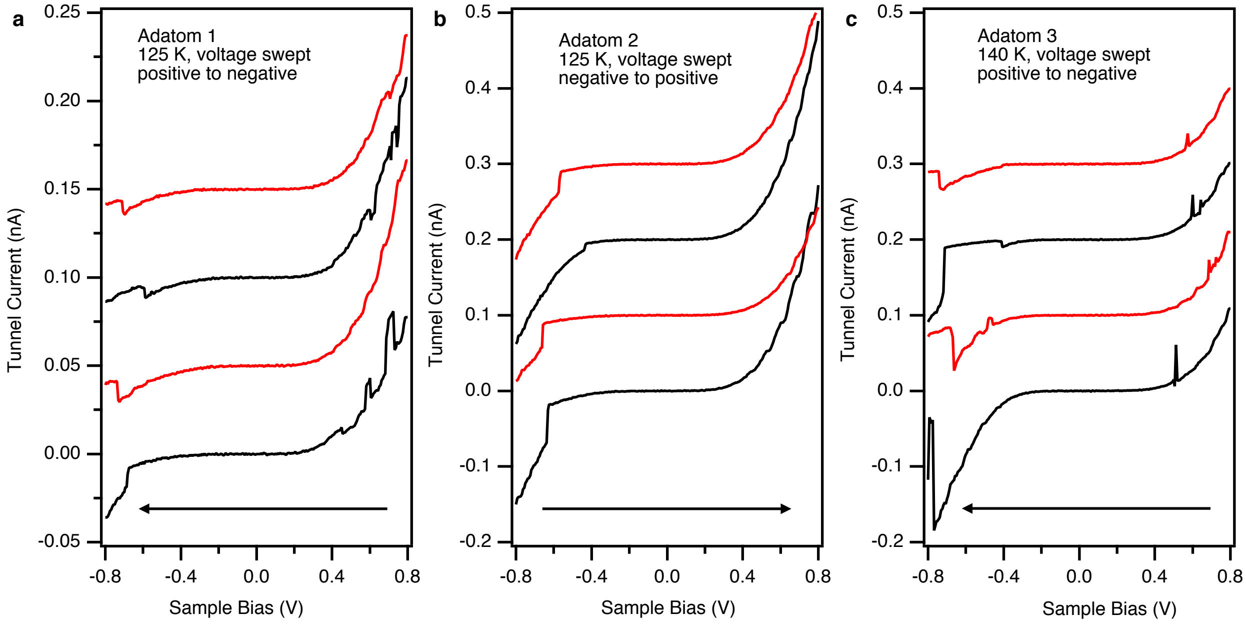


Supplementary Figure S4: **I(V) spectra at bistable adatoms.** (a) Spectra collected at a bistable adatom at 125 K. Successive spectra (obtained by revisiting the same atom in successive imaging sweeps) are offset by 0.05 nA for clarity. Voltage swept positive to negative. (b) Spectra collected at a different bistable adatom at 125 K. Successive spectra are offset by 0.1 nA. Voltage swept negative to positive. (c) Spectra collected at a bistable adatom at 140 K. Successive spectra are offset by 0.1 nA. Voltage swept positive to negative. Tunnel current setpoint is 0.1 nA in all cases, voltage setpoint was +0.8 V. Discontinuities, which include steps and spikes occur at a range of both positive and negative bias voltages, for both sweep directions. Bistability is a recurring phenomenon for the same adatoms even after tip repositioning, although the detailed switching characteristic varies between voltage sweeps. Bistable adatoms have been identified via I(V) spectra at all temperatures studied, from 78 K to 195 K.

## Supplementary Discussion

**Temperature dependence of adatom and vacancy coverage.** Since adatoms on the $PrSr_2Mn_2O_7$ surface are observed to be mobile (figure 6), it is reasonable to ask whether the adatom and vacancy density is constant, or varies with time and sample temperature. A variable temperature STM experiment was therefore performed, and adatom and vacancy coverage extracted by analysis of topographic images. Figures S3a and b show example STM images of $PrSr_2Mn_2O_7$ at 78 K and 195 K. As can be seen from the images, the adatom and vacancy coverage is substantially lower at 195 K than at 78 K. The change in coverage can also be seen in the histograms of these two images, figures S3c and d, with the histogram at 195 K being substantially narrower, indicating a flatter surface. This effect is opposite to what would be expected purely from thermal noise, which would broaden the histogram at higher temperature. To evaluate the coverage of adatoms and vacancies, a cut-off value of $\pm$ 50 pm was adopted: the adatom coverage is measured as the fraction of the image with Z-values above +50 pm, and the vacancy coverage as the fraction below -50 pm. These cut-off values are illustrated in the histograms in figures S3c and d: the 78 K image has 4.1% adatom and 1.7% vacancy coverage: the 195 K image has 1.4% adatom and 0.8% vacancy coverage. STM images were collected at a range of sample temperatures from 78 K to 195 K: the temperature was slowly increased over a period of eight days. Due to thermal effects it was not possible to study the same area at all temperatures, but all images were obtained from the same region of a cleaved $PrSr_2Mn_2O_7$ sample. To get a measure of the variation in adatom and vacancy coverage, at least six different images were analysed for each temperature point: temperatures where insufficient data were collected to evaluate the range of coverage were excluded from this analysis. All images were calibrated in x, y and z to correct for the change in the piezo coefficients with temperature. Figure S3e shows how the adatom and vacancy coverage varies with sample temperature: error bars represent one standard deviation in coverage. The adatom coverage decreases from 5.3 $\pm$ 1.5 % at 78 K to 1.9 $\pm$ 0.4 % at 195 K, the vacancy coverage decreases from 2.9 $\pm$ 1.2 % to 1.0 $\pm$ 0.2 % in the same interval. It should be noted that as this experiment took place over a period of eight days, the decrease in coverage should be viewed as a combined effect of temperature and time. The decrease in both adatom and vacancy coverage suggests that adatom-vacancy recombination is taking place at the $PrSr_2Mn_2O_7$ surface: if the decrease in the number of adatoms were due to desorption from the surface to the vacuum, no corresponding decrease in vacancy density would be observed. Individual adatom-vacancy recombination events have been observed, as shown in figure 7.

**Temperature dependence of adatom mobility.** Figure 6 in the main body of the paper shows a time series of STM images collected at 170 K, covering 15 minutes. Adatoms are observed to appear and disappear from frame to frame. We may define an adatom mobility as the fraction of visible adatoms appearing or disappearing per frame, when averaged over many frames. Such time series were collected at a range of temperatures as part of the variable temperature experiment described above, and the adatom mobility evaluated for each temperature. Figure S3f shows how the adatom mobility varies with temperature. All other parameters such as image size, tunnel current and applied bias voltage were constant. These data have been normalised for the decreasing adatom density at high temperature to give a mobility as a fraction of the number of visible adatoms. The error bars represent one standard error $\sigma/\sqrt{n}$, where $\sigma$ is the standard deviation of the hopping rate and n is the number of frames the measurement is averaged over. The mobility increases from nearly zero at 78 K to around 7% of visible adatoms at 170 K. It is not possible to accurately establish an activation energy for adatom hopping from these data due to the large uncertainties involved. Nonetheless, a reasonable fit of the form $exp(-E_A/k_bT)$ can be made, as shown in figure S3f. The anomalously low mobility at 195 K has been excluded from this fit. In temperature units $E_A$ is found to be 480 $\pm$ 170 K.
